# Supplementary material for: False Discovery Control in Multiple Testing: A Brief Overview of Theories and Methodologies
Source: arXiv:2411.10647 source file (2024-11-16)
Supplement: Supplementary file 1 [file omitted_proofs.tex]

\section{Omitted Technical Details in Main Article}
\subsection{Proof of Theorem \ref{thm:SC}}\label{ap:SC}
	\begin{proof}%[Proof of Theorem \ref{thm:SC}:] 
Suppose that threshold $t_\alpha$ of $\widehat{\rm Lfdr}$-based procedure exists. Then,
	\begin{equation}
		{\rm FDR}(\cR_{t_\alpha})=\EE\biggl[\frac{{\rm FDP}(\cR_{t_\alpha})}{\widehat{\rm FDP}(\cR_{t_\alpha})}\cdot\widehat{\rm FDP}(\cR_{t_\alpha})\biggl]\leq\alpha\cdot\EE\biggl[\frac{{\rm FDP}(\cR_{t_\alpha})}{\widehat{\rm FDP}(\cR_{t_\alpha})}\biggl],
	\end{equation}
	where the inequality results from the threshold choice such that $t_\alpha=\max\{t\in[0,1]:\widehat{\rm FDP}(\cR_{t})\leq\alpha\}$. Thus, in the following proof we will respectively show that: (\romannumeral1) $\EE\left[\frac{{\rm FDP}(\cR_{t_\alpha})}{\widehat{\rm FDP}(\cR_{t_\alpha})}\right]\leq1$ and (\romannumeral2) $t_\alpha$ exists.\\[10pt]
	\textbf{Step 1:} 
	Note that we can decompose the ratio as
	\begin{align*}
	\frac{{\rm FDP}(\cR_t)}{\widehat{\rm FDP}(\cR_t)}&=\frac{\sum_{i=1}^m\ind\big(\widehat{\rm Lfdr}(X_i)\leq t\big)(1-\theta_i)}{\sum_{i=1}^m \ind\big({\rm Lfdr}(X_i)\leq t\big)(1-\theta_i)}\cdot\frac{\sum_{i=1}^m \ind\big({\rm Lfdr}(X_i)\leq t\big)(1-\theta_i)}{\sum_{i=1}^m {\rm Lfdr}(X_i)\ind\big({\rm Lfdr}(X_i)\leq t\big)}\\
	&\qquad\cdot\frac{\sum_{i=1}^m {\rm Lfdr}(X_i)\ind\big({\rm Lfdr}(X_i)\leq t\big)}{\sum_{i=1}^m\ind\big(\widehat{\rm Lfdr}(X_i)\leq t\big)\widehat{\rm Lfdr}(X_i)}.
	\end{align*}
	Following this, we define
	\begin{align}
		D_{m,0}(t)&=\frac{1}{m}\sum_{i=1}^m \ind\big({\rm Lfdr}(X_i)\leq t\big), \quad \widehat{D}_{m,0}(t)=\frac{1}{m}\sum_{i=1}^m \ind\big(\widehat{\rm Lfdr}(X_i)\leq t\big),\nonumber\\
		D_{m,1}(t)&=\frac{1}{m}\sum_{i=1}^m {\rm Lfdr}(X_i)\ind\big({\rm Lfdr}(X_i)\leq t\big),\quad \widehat{D}_{m,1}(t)=\frac{1}{m}\sum_{i=1}^m \widehat{\rm Lfdr}(X_i)\ind\big(\widehat{\rm Lfdr}(X_i)\leq t\big)\nonumber\\
		D_{m,2}(t)&=\frac{1}{m}\sum_{i=1}^m \ind\big({\rm Lfdr}(X_i)\leq t\big)(1-\theta_i), \quad \widehat{D}_{m,2}(t)=\frac{1}{m}\sum_{i=1}^m \ind\big(\widehat{\rm Lfdr}(X_i)\leq t\big)(1-\theta_i)\nonumber
	\end{align}
	Recall that for each $i\in[m]$ the observation follows model in \eqref{eq:bayes_model}:
	$$
	\theta_i\sim{\rm Bernoulli}(\pi),\quad X_i\sim (1-\theta_i)f_{0}+\theta_i f_{1},
	$$
	Following this, based on the Baye's theorem, for all $i\in\cM$, it holds that
	\begin{align}
		&\mathbb{E}_{X_i,\theta_i}\Big[\ind\big({\rm Lfdr}(X_i)\leq t\big)(1-\theta_i)\Big]=\EE_{X_i}\left[\mathbb{E}_{\theta_i|X_i}\Big[\ind\big({\rm Lfdr}(X_i)\leq t\big)(1-\theta_i)\Big]\right]\nonumber\\
		&\qquad=\EE_{X_i}\left[\ind\big({\rm Lfdr}(X_i)\leq t\big)\cdot\PP(\theta_i=0| X_i)\right]=\mathbb{E}_{X_i}\Big[\ind\big({\rm Lfdr}(X)\leq t\big){\rm Lfdr}(X)\Big].
	\end{align}
	Based on the weak law of large numbers, it implies that
	\begin{align}
		\frac{1}{m}\sum_{i=1}^m\ind\big({\rm Lfdr}(X_i)\leq t\big)(1-\theta_i)\overset{p}{\longrightarrow}D_1(t),\quad\frac{1}{m}\sum_{i=1}^m\ind\big({\rm Lfdr}(X_i)\leq t\big){\rm Lfdr}(X_i)&\overset{p}{\longrightarrow}D_1(t),\nonumber
	\end{align}
	where $D_1(t)$ is a continuous function over $[0,1]$. Since $|D_{m,2}-D_{m,1}|\leq|D_{m,2}-D_1|+|D_1-D_{m,1}|$, then $|D_{m,2}-D_{m,1}|\overset{p}{\longrightarrow}0$. Now we are going to show that $|\widehat{D}_{m,1}-{D}_{m,1}|\overset{p}{\longrightarrow}0$ and $|\widehat{D}_{m,2}-{D}_{m,2}|\overset{p}{\longrightarrow}0$. Note that the difference $|\widehat{D}_{m,1}-{D}_{m,1}|$ can be decomposed as
	\begin{align}
		|\widehat{D}_{m,1}-{D}_{m,1}|&\leq\biggl|\frac{1}{m}\sum_{i=1}^m \widehat{\rm Lfdr}(X_i)\ind\big(\widehat{\rm Lfdr}(X_i)\leq t\big)-\frac{1}{m}\sum_{i=1}^m {\rm Lfdr}(X_i)\ind\big(\widehat{\rm Lfdr}(X_i)\leq t\big)\biggl|\nonumber\\
		&\quad+\biggl|\frac{1}{m}\sum_{i=1}^m {\rm Lfdr}(X_i)\ind\big(\widehat{\rm Lfdr}(X_i)\leq t\big)-\frac{1}{m}\sum_{i=1}^m {\rm Lfdr}(X_i)\ind\big({\rm Lfdr}(X_i)\leq t\big)\biggl|\nonumber\\
		&\leq\frac{1}{m}\sum_{i=1}^m\Big|\widehat{\rm Lfdr}(X_i)-{\rm Lfdr}(X_i)\Big|+\frac{1}{m}\sum_{i=1}^m\Big|\ind\big(\widehat{\rm Lfdr}(X_i)\leq t\big)-\ind\big({\rm Lfdr}(X_i)\leq t\big)\Big|\nonumber,
	\end{align}
	where the first term converges to 0 in probability directly follows the weak consistency of $\widehat{\rm Lfdr}(X_i)$. And similarly, $|\widehat{D}_{m,2}-{D}_{m,2}|$ can be written as
	\begin{align}
		|\widehat{D}_{m,2}-{D}_{m,2}|&=\biggl|\frac{1}{m}\sum_{i=1}^m \left[\ind\big(\widehat{\rm Lfdr}(X_i)\leq t\big)-\ind\big({\rm Lfdr}(X_i)\leq t\big)\right](1-\theta_i)\biggl|\nonumber\\
		&\leq\frac{1}{m}\sum_{i=1}^m\Big|\ind\big(\widehat{\rm Lfdr}(X_i)\leq t\big)-\ind\big({\rm Lfdr}(X_i)\leq t\big)\Big|\nonumber.
	\end{align}
	All we left to show is that $\frac{1}{m}\sum_{i=1}^m\big|\ind\big(\widehat{\rm Lfdr}(X_i)\leq t\big)-\ind\big({\rm Lfdr}(X_i)\leq t\big)\big|$ converges to 0 in probability. Note that for any $\epsilon\in(0,1)$, the term can be bounded by
	\begin{align}
		&\frac{1}{m}\sum_{i=1}^m\Big|\ind\big(\widehat{\rm Lfdr}(X_i)\leq t\big)-\ind\big({\rm Lfdr}(X_i)\leq t\big)\Big|\nonumber\\
		&\quad=\frac{1}{m}\sum_{i=1}^m\ind\big({\rm Lfdr}(X_i)\leq t, \widehat{\rm Lfdr}(X_i)> t\big)+\frac{1}{m}\sum_{i=1}^m\ind\big(\widehat{\rm Lfdr}(X_i)\leq t, {\rm Lfdr}(X_i)>t\big)\nonumber\\
		&\quad=\biggl[\frac{1}{m}\sum_{i=1}^m\ind\big(t-\epsilon<{\rm Lfdr}(X_i)\leq t, \widehat{\rm Lfdr}(X_i)> t\big)+\frac{1}{m}\sum_{i=1}^m\ind\big({\rm Lfdr}(X_i)\leq t-\epsilon, \widehat{\rm Lfdr}(X_i)> t\big)\biggl]\nonumber\\
		&\qquad+\biggl[\frac{1}{m}\sum_{i=1}^m\ind\big(t<{\rm Lfdr}(X_i)\leq t+\epsilon, \widehat{\rm Lfdr}(X_i)\leq t\big)+\frac{1}{m}\sum_{i=1}^m\ind\big({\rm Lfdr}(X_i)> t+\epsilon, \widehat{\rm Lfdr}(X_i)\leq t\big)\biggl]\nonumber\nonumber\\
		&\quad\leq\frac{1}{m}\sum_{i=1}^m\ind\big(t-\epsilon<{\rm Lfdr}(X_i)\leq t+\epsilon\big)+\frac{1}{m}\sum_{i=1}^m\ind\left(\left|{\rm Lfdr}(X_i)-\widehat{\rm Lfdr}(X_i)\right|>\epsilon\right)\nonumber\\
		&\quad\leq\Big|D_{m,0}(t+\epsilon)-D_{m,0}(t-\epsilon)\Big|+\frac{1}{m\epsilon}\sum_{i=1}^m\Big|\widehat{\rm Lfdr}(X_i)-{\rm Lfdr}(X_i)\Big|\tag{$\ind(X\geq t)\leq X/t$}.
	\end{align}
	As $\frac{1}{m}\sum_{i=1}^m\Big|\widehat{\rm Lfdr}(X_i)-{\rm Lfdr}(X_i)\Big|\overset{p}{\rightarrow}0$ based on the weak consistency and $\epsilon$ can be arbitrarily small, take limitation at both side and the second term converges to 0 in probability. Then finishes the proof of $|\widehat{D}_{m,1}-{D}_{m,1}|\overset{p}{\longrightarrow}0$ and $|\widehat{D}_{m,2}-{D}_{m,2}|\overset{p}{\longrightarrow}0$. Thus, it holds that
	\begin{align}
		\frac{{\rm FDP}(\cR_t)}{\widehat{\rm FDP}(\cR_t)}&=\frac{\sum_{i=1}^m\ind\big(\widehat{\rm Lfdr}(X_i)\leq t\big)(1-\theta_i)}{\sum_{i=1}^m\ind\big(\widehat{\rm Lfdr}(X_i)\leq t\big)\widehat{\rm Lfdr}(X_i)}=\frac{\widehat{D}_{m,2}(t)}{{D}_{m,2}(t)}\cdot\frac{D_{m,2}(t)}{{D}_{m,1}(t)}\cdot\frac{D_{m,1}(t)}{\widehat{D}_{m,1}(t)}\overset{p}{\rightarrow}1,\nonumber
	\end{align}
	for all $t\in[0,1]$ based on the Slusky's theorem.\\[5pt] 
	\textbf{Step 2:} Recall that there exists constant $t_\infty\in(0,1]$ such that $D_1(t_\infty)/D_0(t_\infty)\leq\alpha$. Following similar arguments as above, we can show that $D_{m,1}(t_\infty)/D_{m,0}(t_\infty)\leq\alpha+o(1)$ as
	\begin{align}
		|\widehat{D}_{m,0}-{D}_{m,0}|&=\frac{1}{m}\sum_{i=1}^m\Big|\ind\big(\widehat{\rm Lfdr}(X_i)\leq t\big)-\ind\big({\rm Lfdr}(X_i)\leq t\big)\Big|\nonumber\\
		&\leq\Big|D_{m,0}(t+\epsilon)-D_{m,0}(t-\epsilon)\Big|+\frac{1}{m\epsilon}\sum_{i=1}^m\Big|\widehat{\rm Lfdr}(X_i)-{\rm Lfdr}(X_i)\Big|,
	\end{align}
	and thus $|\widehat{D}_{m,0}-{D}_{m,0}|\overset{p}{\longrightarrow}0$. Furthermore, we have
	\begin{align}
		\left|\frac{D_{m,1}(t_\infty)}{D_{m,0}(t_\infty)}-\frac{\widehat{D}_{m,1}(t_\infty)}{\widehat{D}_{m,0}(t_\infty)}\right|&\leq\frac{|\widehat{D}_{m,0}(t_\infty)-D_{m,0}(t_\infty)|+|D_{m,1}(t_\infty)-\widehat{D}_{m,0}(t_\infty)|}{|D_{m,0}(t_\infty)\widehat{D}_{m,0}(t_\infty)|}\nonumber\\
		&\leq\frac{|\widehat{D}_{m,0}(t_\infty)-D_{m,0}(t_\infty)|+|D_{m,1}(t_\infty)-\widehat{D}_{m,0}(t_\infty)|}{D_{m,0}(t_\infty)(D_{m,0}(t_\infty)-|\widehat{D}_{m,0}(t_\infty)-D_{m,0}(t_\infty)|)}.
	\end{align}
	Since $D_{m,0}(t_\infty)>0$ as $D_{m,0}(0)=0$, $t_\infty>0$ and $D_{m,0}$ is monotone increasing, then ${\widehat{D}_{m,1}(t_\infty)}/{\widehat{D}_{m,0}(t_\infty)}\\\overset{p}{\rightarrow}{{D}_{m,1}(t_\infty)}/{{D}_{m,0}(t_\infty)}$. Recall that $\widehat{\rm FDP}(t_\infty)={\widehat{D}_{m,1}(t_\infty)}/{\widehat{D}_{m,0}(t_\infty)}\leq\alpha+o(1)$, thus  $t_\alpha=\max\{t\in[0,1]:\widehat{\rm FDP}(\cR_{t})\leq\alpha\}$ exists in probability. Combine Step 1 and Step 2, then we finish the proof.
	\end{proof}

\subsection{Proof of Theorem \ref{thm:GBC}}\label{ap:GBC}
\begin{proof}%[Proof of Theorem \ref{thm:GBC}]
	The proof is akin to that of Theorem \ref{thm:BC} with an explicit construction. For notational simplicity, we write $T_i=\cA(X_i,s_i)$, function $c_i:=c_{s_i}$ and $ S_i=c_i(T_i)$,
	 then we have
	$$
	\begin{aligned}
		\text{FDR}(\cR_{t_\alpha})&=\mathbb{E}\Bigg[\frac{\sum_{i\in\cH_0}\ind(T_i\leq t_{\alpha})}{ \sum_{i=1}^m\ind(T_i\leq t_{\alpha}) \vee1 }\Bigg]\\
		&\leq\mathbb{E}\Bigg[\frac{\sum_{i\in\cH_0}\ind(T_i\leq t_{\alpha})}{ 1+\sum_{i\in\cH_0}\ind( S_i\geq 1-c_i(t_{\alpha}))}\cdot\frac{1+\sum_{i=1}^m\ind(S_i\geq 1-c_i(t_{\alpha})) }{ \sum_{i=1}^m\ind(T_i\leq t_{\alpha}) \vee1 }\Bigg]\\
		&\leq\alpha\cdot\mathbb{E}\Bigg[\frac{\sum_{i\in\cH_0}\ind(T_i\leq t_{\alpha})}{ 1+\sum_{i\in\cH_0}\ind( S_i\geq 1-c_i(t_{\alpha}))}\Bigg],
	\end{aligned}
	$$
	where the first inequality is based on $\sum_{i\in\cH_0}\ind( S_i\geq 1-c_i(t_{\alpha}))\leq\sum_{i=1}^m\ind( S_i\geq 1-c_i(t_{\alpha})) \}$ and the last inequality follows from the choice of $t_{\alpha}$. Then, we only need to show
	\begin{equation}
	\mathbb{E}\Bigg[\frac{\sum_{i\in\cH_0}\ind(T_i\leq t_{\alpha})}{ 1+\sum_{i\in\cH_0}\ind( S_i\geq 1-c_i(t_{\alpha}))}\Bigg]\leq1.
	\end{equation}
	The inequality can be proved using Lemma \ref{lem:BC_optional} through a stopping time argument. Define
	$$
	\breve{T}_i =
	\begin{cases}
		c_i^{-1}(S_i)& \text{ if $S_i\leq0.5$ } \\
		c_i^{-1}(1-S_i)& \text{ if $S_i>0.5$ }. \\
	\end{cases}
	$$
	Let $\breve{\mathcal{T}}=\{\hat{T}_i:i\in\cH_0\}$. 
	Define the order statistics as $\breve{T}_{(1)}\leq\dots\leq\breve{T}_{(m_0)}$, where $m_0=|\cH_0|$. Without loss of generality, assume that the first $|\cH_0|$ hypotheses are null, i.e., $\cH_0=\{1,\dots,|\cH_0|\}$. Consider optional stopping time $J=\max\{j\in\cH_0: \breve{T}_{(j)}\leq t_{\alpha}\}$, where $J$ must exist since $c_i(\breve{T}_i)\leq0.5$ for all $i$ based on the definition, and
	$t_{\alpha}\leq t_{\max}={\rm max}\{t:c_i(t)\leq0.5\text{~for all i}\}$ such that  $c_i(t_\alpha)\leq0.5$ holds. Following this, we can get
	\begin{align}
		\frac{\sum_{i\in\cH_0}\ind(T_i\leq t_{\alpha})}{ 1+\sum_{i\in\mathcal{H}_0}\ind(S_i\geq 1-c_i(t_{\alpha}))}
		&=\frac{\sum_{i\in\mathcal{H}_0}\ind(c_i^{-1}(S_i)\leq t_{\alpha})}{ 1+\sum_{i\in\mathcal{H}_0}\ind(c_i^{-1}(1-S_i)\leq t_{\alpha})}.
		\label{eq:GBC_optional}
	\end{align}
	Let $B_i=\mathds{1}(S_{(i)}>0.5)$ for all $i\in\cH_0$ and
	the order of $S_{(i)}$'s is inherited from $\breve{T}_{(i)}$'s, rather than the magnitude of $S_i$'s. Note that for all $i\in\cH_0$, $c_i^{-1}(S_i)\leq t_{\alpha}$ if and only if $\breve{T}_i\leq t_\alpha$ and $S_{i}\leq0.5$, i.e., $i\leq J$ and $B_i=0$. Similarly,  $c_i^{-1}(1-S_i)\leq t_{\alpha}$ if and only if $\breve{T}_i\leq t_\alpha $ and $S_i>0.5$, i.e., $i\leq J$ and $B_i=1$. Combine the arguments above, \eqref{eq:GBC_optional} can be equivalently written as
	$$
	\frac{\sum_{i\in\cH_0}\ind(T_i\leq t_{\alpha})}{ 1+\sum_{i\in\mathcal{H}_0}\ind(S_i\geq 1-c_i(t_{\alpha}))}
		=\frac{(1-B_1)+\dots+(1-B_J)}{1+B_1+\dots+B_J}=\frac{1+J}{1+B_1+\dots+B_J}-1,
	$$ 
	 Since $B_i$ are independent random variables satisfying $B_i\sim \text{Bernoulli}(0.5)$, by the optional stopping lemma in Lemma \ref{lem:BC_optional}, we have $\mathbb{E}\left[\frac{1+J}{1+B_1+\dots+B_J}\right]\leq 2$, which completes the proof.
\end{proof}
