# Supplementary material for: False Discovery Control in Multiple Testing: A Brief Overview of Theories and Methodologies
Source: arXiv:2411.10647 source file (2024-11-16)
Supplement: Supplementary file 2 [file supp_background.tex]

\section{Supplementary Background}\label{ap:additional}
\subsection{Multiplicity-Related Error Rates}\label{ap:add_error_rates}
\textbf{Recap of Error Rates in Single Testing.} When conducting a hypothesis test, there are two kinds of errors: reject a null hypothesis when it is true (Type \uppercase\expandafter{\romannumeral1} error) or fail to reject a null hypothesis when it is false (Type \uppercase\expandafter{\romannumeral2} error). Type \uppercase\expandafter{\romannumeral1} error occurs when a non-existent pattern is identified in the data (false discovery), while Type \uppercase\expandafter{\romannumeral2} error occurs when an actual pattern goes unnoticed (missed discovery). In practice, it is impossible to eliminate the risk of making decision errors. However, the consequences of these errors usually differ, with Type \uppercase\expandafter{\romannumeral1} error considered a more serious mistake. The rates of Type \uppercase\expandafter{\romannumeral1} and Type \uppercase\expandafter{\romannumeral2} errors are defined as probabilities of making these errors. In the classical single hypothesis testing, the goal is to control the Type \uppercase\expandafter{\romannumeral1} error rate at a pre-specified level $\alpha$ while minimizing the Type \uppercase\expandafter{\romannumeral2} error rate, i.e., maximizing the testing power.\\[10pt]
\textbf{Error Rates in Multiple Testing.} In the multiple testing setting, it is desirable to assess the overall performance of a testing procedure by combining all decisions. For instance, FDR and TDR, as defined in equations \eqref{eq:fdr} and \eqref{eq:tdr}, respectively, provide one kind of measurement for Type \uppercase\expandafter{\romannumeral1} and Type \uppercase\expandafter{\romannumeral2} errors in some sense. The selection of an error rate in applications hinges on the specific purpose of the inference \citep{benjamini2010simultaneous}. Please refer to Table \ref{table:error} for a detailed comparison.
\begin{table}[!htb]%[pos=h] %cols=4,pos=h
        \begin{center}
            \begin{tabular}{@{}lcc@{}}
            \toprule
            \textbf{Error Rates} & \textbf{Abbr.} & \textbf{Expression}   \\ 
            \midrule
            \textbf{Per-Comparison Error Rate} & FCER & $\EE[|\cR\cap\cH_0|/m]\leq\alpha$ \\[10pt]
            \textbf{Per-Family Error Rate} & PFER & $\EE[|\cR\cap\cH_0|]\leq k$ \\[10pt]
            \textbf{Familywise Error Rate}& FWER & $\PP(|\cR\cap\cH_0|\geq1)\leq\alpha$ \\
            $k$-Familywise Error Rate & $k$-FWER & $\PP(|\cR\cap\cH_0|\geq k)\leq\alpha$ \\[10pt]
            \textbf{False Discovery Rate} & FDR & $\EE[|\cR\cap\cH_0|/|\cR|\vee1]\leq\alpha$\\
            $k$-False Discovery Rate & $k$-FDR & $\EE[(|\cR\cap\cH_0|-k)_+/|\cR|\vee1]\leq\alpha$ \\
            Marginal FDR & mFDR & $\EE[|\cR\cap\cH_0|]/\EE[|\cR|\vee1]\leq\alpha$  \\
            Positive FDR & pFDR & $\EE[|\cR\cap\cH_0|/|\cR|\vert|\cR|>0]\leq\alpha$ \\
            False Discovery Exceedance & ${\rm FDX}_\tau$ & $\PP(|\cR\cap\cH_0|/|\cR|\geq\tau)\leq\alpha$ \\
            Weighted FDR & wFDR & $\EE\big[\sum_{i\in\cH_0}\omega_i\ind(i\in\cR)/\sum_i\omega_i\ind(i\in\cR)\vee1\big]\leq\alpha$ \\
            \bottomrule
        \end{tabular}
        \caption{List of multiplicity-related error rates for simultaneous and selective inference.}
        \label{table:error}
        \end{center}
    \end{table}
    
Specifically, PCER and PFER are two unadjusted error measures, measuring the expectation of Type \uppercase\expandafter{\romannumeral1} errors. FWER (\emph{strong control}, see \S\ref{ap:fewr_method} for discussion), a well-established concept, is defined as the probability of making at least one Type \uppercase\expandafter{\romannumeral1} error in the family. It provides a solution for various statistical scenarios and purposes, including regulation, policy-making, and scientific reporting. However, the drawback is that FWER control significantly limits the power of statistical methods, making it only advisable to use when \emph{simultaneous inference} is essential. An extension of FWER is the $k$-FWER \citep{romano2005testing}, characterizing the probability of committing $k$ or more Type \uppercase\expandafter{\romannumeral1} errors within the family. In comparison, controlling FDR \citep{benjamini1995controlling} safeguards against selection effects but lacks simultaneous inference. Due to its effective error measure adjusted on false rejections and the significant power of correspondence methods, FDR has emerged as one of the most widely adopted error rates.  Besides, together the with False Coverage Rate (FCR), it can provide advanced testing methods and reliable confidence intervals. This makes it a suitable objective for gene filtration and feature selection. Similar to $k$-FWER, the extension of $k$-FDR \citep{Sarkar2009OnAG} allows personal assessment of the implications of relaxing the requirements of FDR. Besides, mFDR and pFDR are variations on FDR, serving as important intermediate statistics (see Theorem \ref{prop:fdrmfdr}). \cite{Genovese2004ASP} introduced FDX as a more robust version of FDR, especially when the FDPs are highly variable. wFDR \citep{benjamini1997multiple} is a promising, yet less-explored approach. With external weights indicating the monetary value, it allows selective inference that can integrate more prior knowledge. Additionally, it serves regulatory purposes, particularly for controlling the selection effects of secondary endpoints within clinical trials. To summarize, the practitioners should match error rates to inference needs.

\subsection{Controlling Methodologies for FWER}\label{ap:fewr_method}
An extensive review of the FWER and $k$-FWER methodologies can be respectively found in \cite{shaffer1995multiple} and \cite{Sarkar2007STEPUPPC}. In this subsection, we present the two most celebrated methodologies --- Bonferonni's method and Holm's procedure. Before delving into the details, we provide clarification on the definition of different control levels of FWER.  We say a testing procedure controls FWER \emph{weakly} if it controls the FWER under the \emph{global null}, i.e., $\cH_0=\cM$. However, discussions among statisticians primarily revolve around FWER control in the strong sense, i.e., $\cH_0\subseteq\cM$. In the following, we first provide some arguments about the relationship between FDR and FWER.
\begin{proposition}
	(\romannumeral1) ${\rm FDR}(\cR)={\rm FWER}(\cR)$ if $\cH_0=\cM$; (\romannumeral2) ${\rm FDR}(\cR)\leq{\rm FWER}(\cR)$.
	\label{prop:FWER_FDR}
\end{proposition}
\begin{proof}[Proof of Proposition \ref{prop:FWER_FDR}]
	Under the global null where $\cH_0=\cM$, any rejection is a false rejection. Following this, we have ${\rm FDP}(\cR)\in\{0,1\}$. Thus, it holds that
	$$
	{\rm FDR}(\cR)=\PP({\rm FDP}(\cR)=1)=\PP(|\cR\cap\cH_0|\geq1)={\rm FWER}(\cR).
	$$
	Similarly, we have
	$$
	{\rm FDR}(\cR)=\EE[{\rm FDP}(\cR)\ind(|\cR\cap\cH_0|\geq1)]\leq\PP(|\cR\cap\cH_0|\geq1)={\rm FWER}(\cR),
	$$
	where the first equation follows ${\rm FDP}(\cR)={\rm FDP}(\cR)\ind(|\cR|\geq1)={\rm FDP}(\cR)\ind(|\cR\cap\cH_0|\geq1)$.
\end{proof}
Proposition \ref{prop:FWER_FDR} yields two noteworthy conclusions: (\romannumeral1) all FDR-controlled methodologies exert a weak control over FWER, and (\romannumeral2) FDR control is less stringent, meaning that if the metric aligns with objectives, opting to control FDR rather than FWER will offer greater statistical power. Next, we introduce the two most celebrated FWER-controlled procedures.

\paragraph{Bonferonni's Method.} Bonferonni's method for multiple hypotheses testing rejects all hypotheses with p-value below threshold $\frac{\alpha}{m}$. The method ensures FWER control in a strong sense, following:
$$
\PP(|\cR_{t_\alpha}\cap\cH_0|\geq1)\leq\EE|\cR_{t_\alpha}\cap\cH_0|\leq\sum_{i\in\cH_0}\PP\left(P_i\leq\frac{\alpha}{m}\right)=\frac{|\cH_0|}{m}\alpha.
$$
We remark that Bonferonni's method is valid for dependent p-values. If we assume independence, then we could employ the Sidak's procedure by choosing threshold as $\alpha_m=1-(1-\alpha)^\frac{1}{m}$, since
$$
\PP(|\cR_{t_\alpha}\cap\cH_0|\geq1)=1-\PP(|\cR_{t_\alpha}\cap\cH_0|=0)=1-(1-\alpha_m)^{|\cH_0|}\leq\alpha.
$$
\paragraph{Holm's Procedure.} The intuition behind Holm's procedure is that p-values can at least jointly provide information about $|\cH_0|$ and thus the procedure can be adjusted on the number of rejections to improve the statistical power. In short, Holm's procedure follows that
\begin{equation}
\textbf{Holm's:}\quad T_i=P_i,\quad t_\alpha=\min\left\{m+1-\sum_{i\in\cM}\ind(P_i\leq t)>\frac{\alpha}{t}\right\},
\end{equation}
and choose rejection set as $\cR_{t_\alpha}$. Then, we provide the theoretical guarantee of Holm's procedure.
\begin{theorem}
	 Holm's procedure at level $\alpha\in (0,1) $ controls FWER at $\alpha $ in finite sample.
	 \label{thm:holm}
\end{theorem}
\begin{proof}[Proof of Theorem \ref{thm:holm}]
	Suppose that Holm's procedure commits at least one false rejection. Following the threshold choice of Holm's procedure in \eqref{eq:holm_threshold}, then we have
	\begin{equation}
	t_\alpha\leq\frac{\alpha}{m+1-\sum_{j\in\cM}\ind(P_j\leq t_\alpha)}\leq\frac{\alpha}{m+1-\sum_{j\in\cM}\ind(P_j\leq \min_{i\in\cH_0}P_i)}\leq\frac{\alpha}{|\cH_0|},
	\label{eq:holm_threshold}
	\end{equation}
	where the second inequality results from $\min_{i\in\cH_0}P_i\leq t_\alpha$ due to the existence of the false rejections, and the second inequality arises from
	$$
	\sum_{j\in\cM}\ind\left(P_j\leq \min_{i\in\cH_0}P_i\right)=\sum_{j\in\cH_1}\ind\left(P_j\leq \min_{i\in\cH_0}P_i\right)+1\leq m-|\cH_0|+1.
	$$
	Following \eqref{eq:holm_threshold} and taking a union bound over the set of null hypotheses $\cH_0$, it holds that
	$$
	{\rm FWER}(\cR_{t_\alpha})=\PP(|\cR_{t_\alpha}\cap\cH_0|\geq1)=\PP\left(\min_{i\in\cH_0}P_i\leq t_\alpha\right)\leq\PP\left(\min_{i\in\cH_0}P_i\leq\frac{\alpha}{|\cH_0|}\right)\leq\alpha.
	$$
\end{proof}
Holm's procedure does not require independence of the p-values and strictly dominates the Bonferroni procedure. Please refer to \cite{hochberg1987multiple} for an extensive review of FWER methodologies.

\subsection{Storey's Adaptive Procedure}\label{ap:storey}
In \S\ref{sec:BC}, we demonstrated that Storey's $\hat{\pi}_0$ effectively addresses the over-conservativeness of the BH procedure. Here, we make a supplement argument about the Storey's $\hat{\pi}_0(\lambda)$-adaptive procedure. As shown in \cite{storey2004strong}, finite-sample control guarantee is attainable with slight modification:
\begin{equation}
\textbf{Storey's:}\quad T_i=P_i,\quad \widehat{\rm FDP}(t)=\frac{\hat{\pi}_0(\lambda)\cdot mt}{\sum_{i=1}^m\ind(P_i\leq t)},
\end{equation}
where Storey's $\hat{\pi}_0$ is defined in \eqref{eq:storeypi} and the slight modification lies in the choice of candidate threshold set such $t_\alpha=\sup\{t\in(0,1-\lambda]:\widehat{\rm FDP}(t)\leq\alpha\}$. The following theorem demonstrates that Storey's procedure ensures a finite-sample FDR control for all fixed $\lambda\in(0,1)$.
 \begin{theorem}\label{thm:storey}
 Storey's procedure controls FDR at $\alpha$ in finite-sample.
 \end{theorem}
 
 \begin{proof}[Proof of Theorem \ref{thm:storey}]
 	For $t\in [0,1]$, denote $ F(t)=|\cR_t\cap\cH_0| $.  Note that
 	\begin{align}
 		{\rm FDR}(\cR_{t_\alpha})&=\EE\biggl[\frac{{\rm FDP}(t_\alpha)}{\widehat{\rm FDP}(t_\alpha)}\cdot\widehat{\rm FDP}(t_\alpha)\biggl]\leq\alpha(1-\lambda)\cdot\EE\left[\frac{F(t_\alpha)}{t_\alpha\left(1+\sum_{i\in\cM}\ind\left(P_i\geq\lambda\right)\right)}\right],
 	\end{align}
 	 where the inequality results from threshold choice such that $\widehat{\rm FDP}(t_\alpha)\leq\alpha$. Write $S_\lambda=\{\ind(P_i\geq\lambda)\}_{i\in\cM}$ given $\lambda\in(0,1)$. Furthermore, based on the double expectation theorem, we can get
 	 \begin{align}
 		\EE\left[\frac{F(t_\alpha)}{t_\alpha\left(1+\sum_{i\in\cM}\ind\left(P_i\geq\lambda\right)\right)}\right]=\EE\left[\frac{1}{1+\sum_{i\in\cM}\ind\left(P_i\geq\lambda\right)}\cdot\EE\left[\frac{F(t_\alpha)}{t_\alpha}\ \biggl\vert\ S_\lambda\right]\right].
 	\end{align} 
 	 For any threshold $t\in [0,1-\lambda]$, we define the filtration as $\mathcal F_t =\sigma \{(\ind(P_1\le \tau),\dots, \ind(P_m\le \tau)): \tau\in [ t,1-\lambda]\}$. Following this, for all $\tau\leq t$, it holds that
 	 \begin{align}
 		&\EE\left[F(\tau)\mid \cF_t,S_\lambda\right]= \sum_{i\in\cH_0}\mathbb{E}\left[\ind(P_i\le \tau) \mid \mathcal F_t,S_\lambda\right]\nonumber \\
 		&\quad=\sum_{i\in\cH_0}\mathbb{E}\left[\ind(P_i\le \tau) \mid \ind(P_i\le t),\ind\left(P_i\geq\lambda\right)\right] = \sum_{i\in\cH_0}\frac{\tau}{t}\ind(P_i\le t)=\frac{\tau}{t}F(t).
 		\label{eq:storey_martingale}
 	\end{align}
 	Notes that \eqref{eq:storey_martingale} indicates that $\mathbb{E}[F(\tau)/\tau|\mathcal F_t]=F(t)/t$ and thus $ t\mapsto F(t)/t$ is still a backward martingale \emph{conditioned on $S_\lambda$} (compared with the martingale arguments in Theorem \ref{thm:BH}).
Furthermore,  $t_\alpha$ is a stopping time with respect to the filtration  $(\mathcal F_t)_{t\in [0,1-\lambda]}$, and the optional stopping theorem \citep{grimmett2020probability} gives that
$\mathbb{E}[F(t_\alpha)/t_\alpha] =F(1-\lambda)$. Following this, we have
\begin{align*}
 		{\rm FDR}(\cR_{t_\alpha})&\leq\frac{\alpha(1-\lambda)}{\lambda}\cdot\EE\left[\frac{\sum_{i\in\cH_0}\ind(P_i\leq1-\lambda)}{1+\sum_{i\in\cH_0}\ind\left(P_i\geq\lambda\right)}\right]\\
 		&=\frac{\alpha(1-\lambda)}{\lambda}\cdot\EE\left[\frac{\sum_{i\in\cH_0}\ind(P_i\leq1-\lambda)}{1+|\cH_0|-\sum_{i\in\cH_0}\ind\left(P_i\leq1-\lambda\right)}\right]\leq(1-\lambda^{|\cH_0|})\cdot\alpha,
 	\end{align*}
 	where the last inequality results from $\sum_{i\in\cH_0}\ind\left(P_i\leq1-\lambda\right)\sim{\rm Binom}(|\cH_0|,1-\lambda)$.
 \end{proof}
 We remark that while Storey's procedure effectively mitigates the overconservativeness of the BH procedure under general scenarios, similar to the BC procedure, it does not consistently outperform the BH procedure, particularly in cases of weak feature signals. Additionally, the proof of Theorem \ref{thm:storey} can be seen as a simplified version of the proof for the BC procedure with fixed $\lambda$.

\subsection{Testing with Conformal P-Values}\label{ap:conformal_p}
Following \cite{bates2023testing}, we discuss the conformal p-values under the outlier detection framework. Suppose that the practitioner observes a dataset $\cD=\{X_i\}_{i\in\cN}$ that contains $n$ independent and independent and identically distributed points $X_i\in\RR^d$ drawn from an unknown distribution $\cP_X$, and conformity score function $s:\RR^d\mapsto\RR$ is decided beforehand to measure how much a new observation conforms to previous data. For instance, a smaller value of $s(X)$ may provide stronger evidence that $X$ is an outlier. Typically, such a conformity score function is trained by partitioning the observations into training and calibration data $\mathcal{D}=\mathcal{D}_{\text{test}}\cup\mathcal{D}_{\text{cal}}$, and train $s=\hat{s}(\cD_{\rm test})$. Given testing data $X_{n+1},\dots,X_{n+m}$, the objective is to test $H_{0,i}:X_{n+1}\sim\cP_X$ for all $i\in\{n+1,\dots,n+m\}$. For any $X\in\RR^d$, the conformal p-value is defined as below:
\begin{equation}
	u(X;\cD)=\frac{1+|\{i\in\cN:s(X_i)\leq s(X)\}|}{n+1}.
	\label{eq:conformal_p}
\end{equation}
For notational simplicity, we write $P_i=u(X_i)$ for all $i\in\{n+1,\dots,n+m\}$. \cite{vovk1999machine} has shown that for all $X\sim\cP_X$, $u(X)$ is a \emph{marginally} super-uniform p-value such that
\begin{equation}
\PP\left(u(X;\cD)\leq t\right)\leq t,\quad \forall t\in(0,1),
\label{eq:marginal_super_uniform}
\end{equation}
where the randomness is introduced by $X$ and observations $\cD$. Equibalently, $u(X,\cD)$ is uniformly distributed on $\left\{\frac{1}{n+1},\dots,\frac{n}{n+1},1\right\}$. Given the definition of marginal p-values in \eqref{eq:conformal_p}, it should be intuitive that larger scores in $\cD$ make the p-values for all test data simultaneously smaller, and vice-versa. Thus, conformal p-values shall share some kind of positive correlations, and this intuitive idea is formalized by the following result proving conformal p-values are PRDS.
\begin{theorem}
	Assume that $u(\cdot)$ is continuously distributed. Then, the conformal p-values $(P_i)_{i\in\cM}$ in correspondence to $X_{n+1},\dots,X_{n+m}$ are PRDS on the set of true nulls hypotheses $\cH_0$.
	\label{thm:conformal_p}
\end{theorem}
\begin{proof}%[Proof of Theorem \ref{thm:conformal_p}]
	Let $S_i=s(X_{i})$ be the conformality scores for all $i\in[n+m]$ and $\Pb=(P_1,\dots,P_m)$ be the conformal p-values evaluated on observations $\cD$. Furthermore, we define $Z_i=(\Sbb_{(i)}',\Sbb_{-i})$, where $\Sbb_{-i}=(S_{n+1},\dots,S_{n+i-1},S_{n+i+1},\dots,S_{n+m})$ and $\Sbb_{(i)}'=(S_{(1)}',\dots,S_{(n+1)}')$ denotes the order statistics of $(S_1,\dots,S_n,S_{n+i})$. Note 
	\begin{align*}
	\left\{\left(S_{(1)},\dots,S_{(n)}\right)\mid P_i,\Sbb_{(i)}'\right\}&{=}\left\{\left(S_{(1)},\dots,S_{(n)}\right)\mid R_i,\Sbb_{(i)}'\right\}\\
	&\overset{d}{=}\left(S_{(1)}',\dots,S_{(R_i-1)}',S_{(R_i+1)}'\dots,S_{(n+1)}'\right),
	\end{align*}
where $R_i$ is the rank of $S_{n+i}$ among $(S_1,\dots,S_n,S_{n+i})$ suggested by $P_i$. Intuitively, the preceding argument suggests that $P_i$ and $Z_i$ suffice to provide the order statistics $(S_{(1)},\dots,S_{(n)})$ of $(S_1,\dots,S_n)$, implying that $P_j$ is jointly \emph{determined} by $P_i$, $Z_i$, and $S_{n+j}$.  Thus, $\Pb=(P_1,\dots,P_m)$ is a deterministic function of $P_i$ and $Z_i$, denoted by $\Pb=G(P_i,Z_i)$. Given $Z_i$, for $j\neq i$ it holds that
\begin{align*}
G_j(P_i,Z_i)&=\frac{1}{n+1}\left(1+\sum_{k\neq R_i,k\leq n+1}\ind\left(S_{n+j}\geq S'_{(k)}\right)\right)\\
&=\frac{1}{n+1}\left(1-\ind\left(S_{n+j}\geq S'_{(R_i)}\right)+\sum_{k=1}^{n+1}\ind\left(S_{n+j}\geq S'_{(k)}\right)\right). 
\end{align*}
Following this, we have each entry $G_j(P_i,Z_i)$ is increasing in $P_i$ for all $j\neq i$ as $R_i$ is increasing in $P_i$. If $i\in\cH_0$, then $S_{n+i}\mid \Sbb_{(i)}'\sim {\rm Unif}(\Sbb_{(i)}')$ and $P_i$ has the same distribution after conditioning. Thus, $P_i\perp\Sbb_{(i)}'$. Furthermore, since $Z_{n+i}\perp Z_{n+j}$ for all $i\neq j$ by assumption, then $P_i\perp\Sbb_{-i}$. Combine the argument above, we have $P_i\perp Z_i$. For any increasing set $A$, it holds that
\begin{align*}
	\PP(\Pb\in A\mid P_i=p)&=\PP\left(G(p,Z_i)\in A\mid P_i=p\right)\\
	&=\EE_{Z_i}[\PP\left(G(p,z)\in A\mid P_i=p,Z_i=z\right)]=\EE_{Z_i}[\ind\left(G(p,z)\in A\right)].
\end{align*}
Since $A$ is an increasing set, $G_i(p,z)=p$ is non-decresing and $G_j(p,z)$ for all $j\neq i$ are increasing in $p$, then $\ind\left(G(p,z)\in A\right)$ is increasing in $p$, which implies the PRDS property.
\end{proof}
We remark that similar to the argument in \eqref{eq:marginal_super_uniform}, in the proof of Theorem \ref{thm:conformal_p}, we treat observations $\cD$, equivalently $\Sbb_{(i)}'$ in $Z_i$, as random variables. Thus, the conformal p-values in \eqref{eq:conformal_p} only conform to the PRDS property \emph{marginally}. Unfortunately, such a guarantee may be insufficient for a practitioner who needs to compute p-values for a large number of test points but is constrained to working with single observations $\cD$. Fortunately, it has been shown that calibration-conditional conformal p-values are attainable. Please refer to Section 3 in \cite{bates2023testing} for details.
