# Supplementary material for: False Discovery Control in Multiple Testing: A Brief Overview of Theories and Methodologies
Source: arXiv:2411.10647 source file (2024-11-16)
Supplement: Supplementary file 3 [file technical_lemmas.tex]

\section{Technical Lemmas}
\begin{lemma}
		\citep[Lemma 1]{barber2019knockoff} Suppose that $B_1,\dots,B_n$ are independent variables with $B_i\sim {\rm Bernoulli}(\rho_i)$ for each $i$ where ${\rm min}_i\ \rho_i\geq\rho>0$. Let $J$ be a stopping time in reverse time in respect to the filtration $\{\mathcal{F}_j\}$ where
		$$
		\mathcal{F}_j=\{B_1+\dots+B_j,B_{j+1}+\dots+B_{n}\}.
		$$
		Then
		$$
		\mathbb{E}\Bigg[\frac{1+J}{1+B_1+\dots+B_n}\Bigg]\leq\rho^{-1}.
		$$
		\label{lem:BC_optional}
	\end{lemma}
